# Supplementary material for: Space-time approach to microstructure selection in solid-solid transitions
Source: arXiv:1001.3549 source file (2010-01-20)
Supplement: Supplementary file 1 [file supptext.pdf]

# Supplementary text and figure for, 'Spacetime approach to microstructure selection in solid- solid transitions', by Surajit Sengupta, Jayee Bhattacharya and Madan Rao

## I. METHODS

### A. Molecular Dynamics

Our MD simulation is carried out on $N = 12099$ particles in the $NVT$ ensemble with periodic boundary conditions attached to a Nosé-Hoover thermostat [19]. Particles interact via an effective (purely repulsive) short range potential – a sum of an anisotropic 2-body $V_2(\mathbf{r}_{ij}) = v_2\,(\sigma/r_{ij})^{12}\,\{1 + \alpha\cos^2 2\theta_{ij}\}$ and 3- body $V_3(\mathbf{r}_i, \mathbf{r}_j, \mathbf{r}_k) = v_3\,[f_{ij}\sin^2(4\theta_{ijk})f_{jk} + f_{jk}\sin^2(4\theta_{jki})f_{ki} + f_{ki}\sin^2(4\theta_{kij})f_{ij}]$ potentials. Particles $i$ and $j$ are separated by a distance $r_{ij}$, $\theta_{ijk}$ is the bond angle at $j$ between triplets $(ijk)$, and $f_{ij} \equiv f(r_{ij})$ is any short ranged, nonnegative, monotonically decreasing function. The units of length and energy are set by $\sigma$ and $v_2$ respectively, making the unit of time $\sigma\sqrt{m/v_2}$, where $m$ is the particle mass. The molecular dynamics time step (MDS) is chosen to be 0.001 corresponding roughly to a real time of 1 fs. In all the figures we choose $10^3$ MDS as our unit of time and the parameters of the thermostat is fixed throughout.

### B. Definitions of order parameter strain and Non-affine parameter

The order parameter strain is obtained by fitting an affine transformation to the neighborhood of a particle with the untransformed square crystal as reference [8,16]. The non-affine parameter $\phi = \chi^2 \times \mathrm{sgn}(\Delta\rho)$ where $\chi^2$ is the error of the fit and $\Delta\rho$ is the change in local density. Note that in the F phase the large non-affine contribution masks the order parameter strain (Fig. 1 b).

### C. Shape anisotropy and degree of twinning

The shape anisotropy of the nucleus is defined as $A = (\lambda_> - \lambda_<)/(\lambda_> + \lambda_<)$, where $\lambda_>$ and $\lambda_<$ are the eigenvalues of the moment of inertia tensor of the growing nucleus [16]. The degree of twinning can in principle be measured by the amplitude of the appropriate Fourier component of the equal time $e_3$. However, we find it convenient to measure it by the correlation function, $\langle e_3(0,t)e_3(\mathbf{r},t)\rangle$ calculated within a droplet. For a twinned (untwinned) nucleus this has a 2 (4) - fold symmetry and $\Psi_2$ is the 2nd order ($l = 2$) coefficient in a Legendre polynomial expansion of the correlation function.

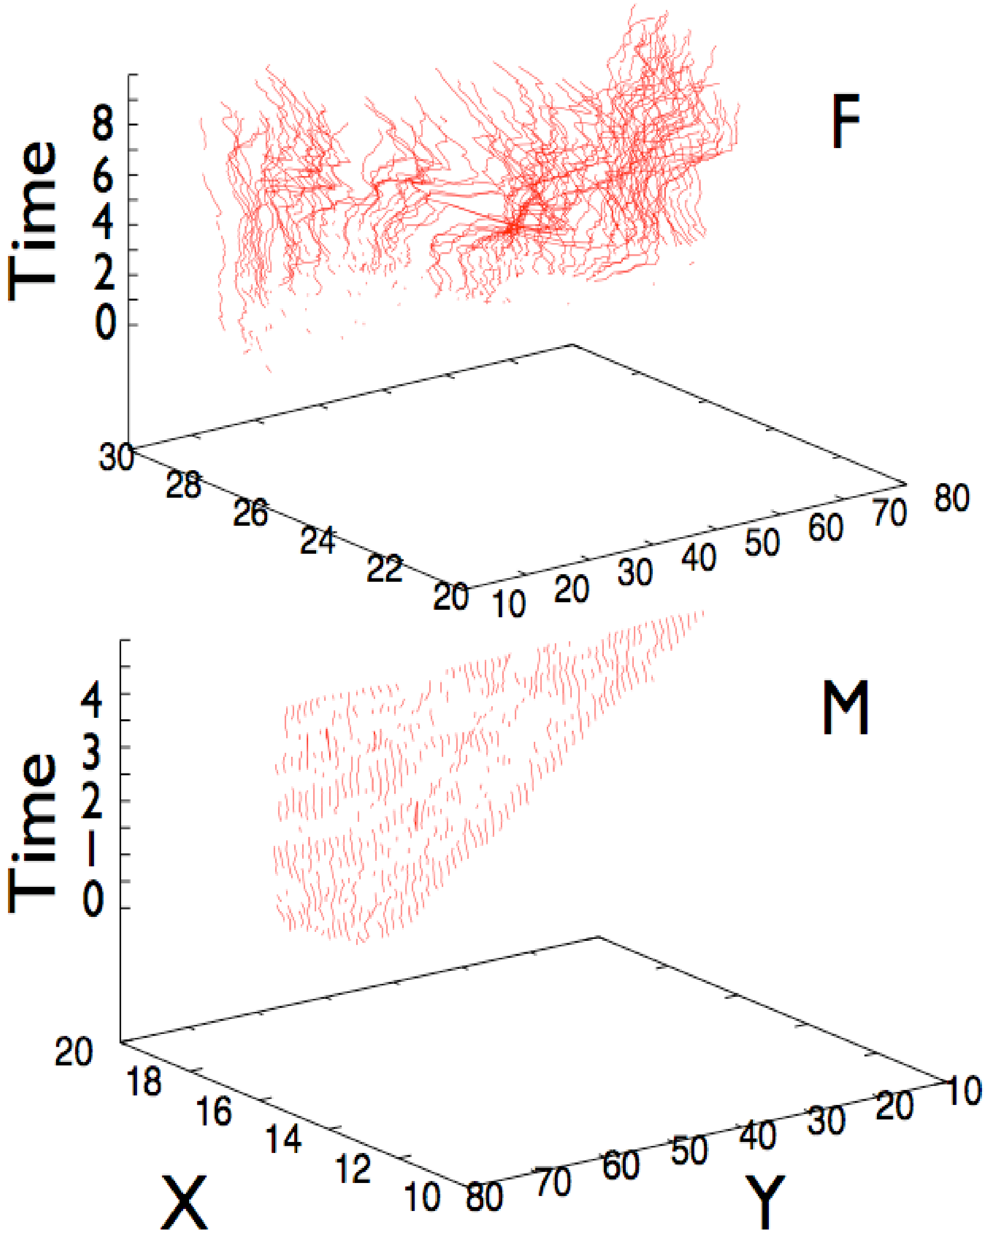


FIG. 1: Space time trajectory plots of active particles (red lines) which belong to a crystalline row at time $t = 0$ in the $F-$ (top, $T = 0.6$) and $M-$ (bottom, $T = 0.1$) phases. Note that the trajectories of particles in the $F-$ phase are disordered and entangled with each other, while those in the $M-$ phase are ballistic and are directed along specific channels. The data shown in this figure is the same as in Fig. 2 (b) in the manuscript, the expanded scale and the full three dimensional representation makes the differences between the $F-$ and the $M-$ phases more prominent in this plot.
